# Supplementary material for: A transport method for restoring incomplete ocean current measurements
Source: arXiv:1808.07965 ancillary file (2018-08-23)
Supplement: Supplementary file 1 [file Supplemental_Materials.pdf]

# Supplemental materials for "A transport method for restoring incomplete ocean current measurements"

Siavash Ameli*[1,2] and Shawn C. Shadden†[1]

[1] *Mechanical Engineering, University of California, Berkeley, CA, USA 94720*
[2] *Department of Mathematics, University of California, Berkeley, CA, USA 94720*

## Datasets

All data that have been used in our manuscript can be found online at *Coastal Observing Research and Development Center* (http://cordc.ucsd.edu/projects/mapping/), which provides real-time and archival access to the HF radars over all US coastlines. For convenience, we have provided both the original and post-processed data (*Ameli and Shadden*, 2018), including

1. Martha's Vineyard HF radar original data
2. Martha's Vineyard HF radar post-processed data
3. Monterey Bay HF radar original data
4. Monterey Bay HF radar post-processed data

## Web-based tool

We have developed a web-based gateway to accompany our manuscript available at http://transport.me.berkeley.edu/restore/ and has been designed to be a community tool to process incomplete oceanographic datasets. The gateway contains a user guide, documentation and sample data–including those that has been used in this manuscript. A brief video of the tool is demonstrated at https://vimeo.com/274810038. All results of this manuscript can be reproduced using our online tool. For instance, in Figure 0.1 we have illustrated the comparison of original and post-processed HF radar data at Monterey Bay, that is computed and visualized with our web-based tool.

## References

Ameli, A., and S. C. Shadden (2018), Restoration of incomplete oceanographic datasets, v2, *UC Berkeley Dash*, doi:https://doi.org/10.6078/D1ZT1M. 1

*Email address: sameli@berkeley.edu
†Email address: shadden@berkeley.edu

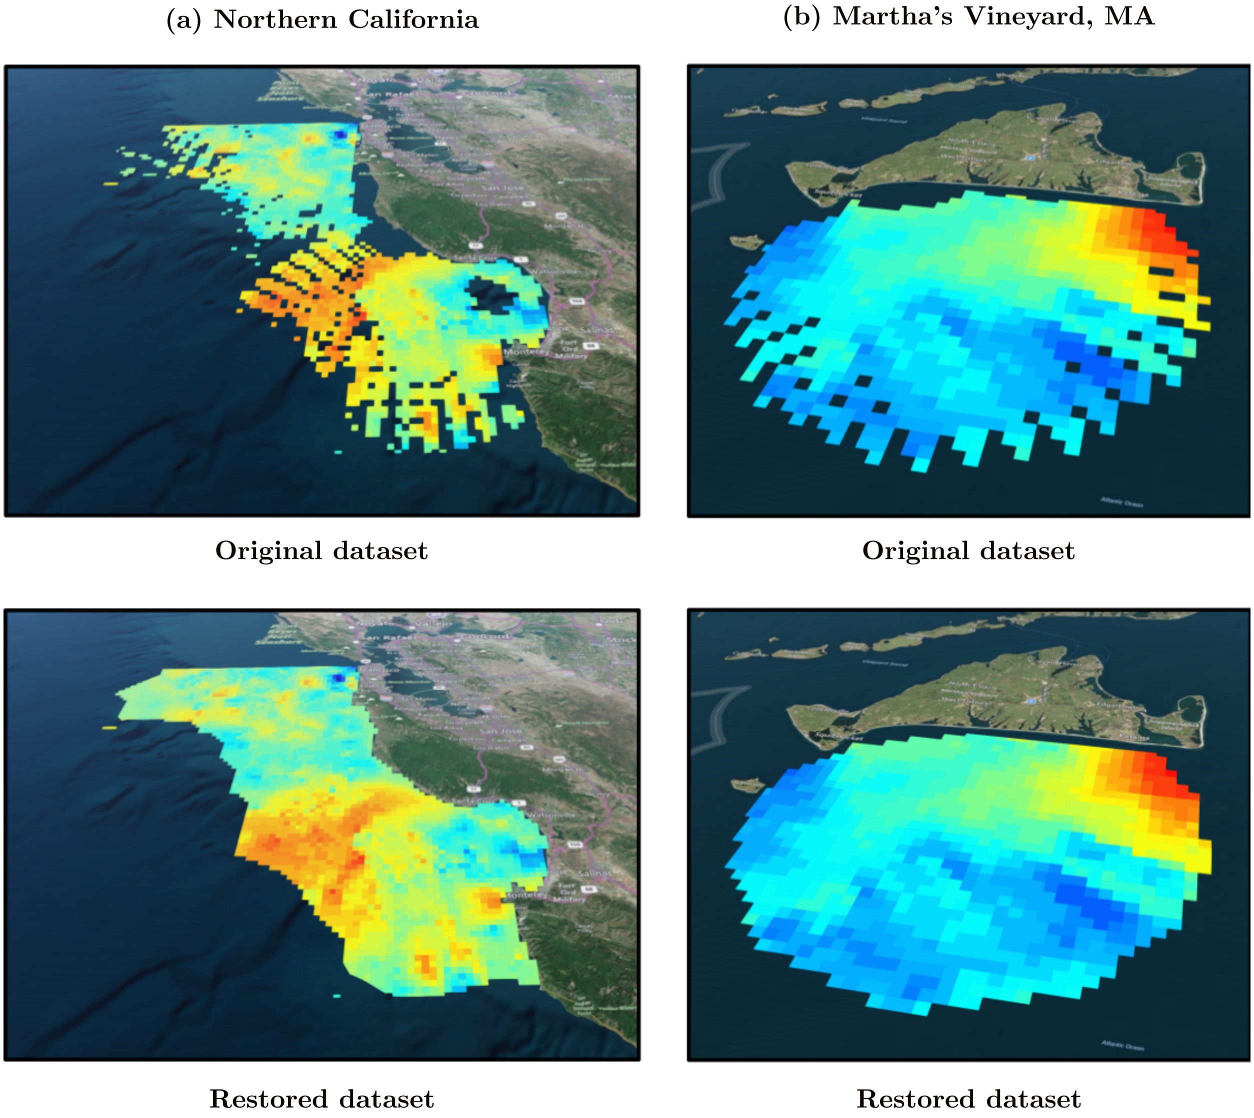


**Figure 0.1:** North component of ocean surface velocity fields obtained from HF radars for (a) northern California and (b) Martha's Vineyard, MA. First rows are the original data and second rows are the restored datasets.
